# Supplementary material for: Sample-based calibration for cryogenic broadband microwave reflectometry measurements
Source: arXiv:1801.00436 source file (2019-07-08)
Supplement: Supplementary file 1 [file supplementaryMat_22062019.pdf]

# SUPPLEMENTARY MATERIAL

## SAMPLE-BASED CALIBRATION FOR CRYOGENIC BROADBAND MICROWAVE REFLECTOMETRY MEASUREMENTS

F. Couëdo[1], L. Bergé[1], L. Dumoulin[1], M. Aprili[2], C.A. Marrache-Kikuchi[1] and J. Gabelli[2]

[1]CSNSM-Centre de Sciences Nucléaires et de Sciences de la Matière, CNRS, Univ. Paris-Sud, Université Paris-Saclay, 91405, Orsay, France

[2]Laboratoire de Physique des Solides, CNRS, Univ. Paris-Sud, Université Paris-Saclay, 91405, Orsay cedex, France

### Microwaves lines

At room temperature, outside the cryostat the microwave lines were cooper cables in order to minimize the losses. Within the cryostat, stainless steel cables have been used between the different temperature stages on the input lines to avoid thermal short-cuts. All microwave coaxial cables were therefore stainless steel ULT-05 cables from Keycom company which have a low heat conduction and low insertion losses. Moreover, the inner conductor of the cryogenic cables needs to be thermalized at each temperature stage of the cryostat. -10dB attenuators are used for this purpose. All connections between the various cables were made using SMA-type connectors. On the sample side, the coaxial geometry is preserved between the commercial coaxial cables and the sapphire substrate thanks to the microstrip geometry (Fig. 3). All microstrip microwave lines have been designed to have a 50 Ω characteristic impedance matching the whole microwave circuitry (input impedance of the amplifiers, ports of the VNA, ...).

### References used for the Standard Calibration (SC)

The accuracy of the SC in our set-up is principally limited by the reproducibility of the SMA connections from one cool-down to the next (see main text). This is why, although some cryogenic microwave calibration kits are commercially available, we have used more conventional standards : at port #3 (see Fig. 2), we have left the incoming microwave line open to create an "Open" standard. For the "Short" reference, we have attached a standard short SMA termination, specified for room temperature operation. For the "Load" reference, we have used a 50 Ω resistance XMA component, which impedance is guaranteed at low temperature [32]. All those standards have been calibrated at room temperature, directly at the output of the VNA, using the Rohde & Schwarz ZV Z135 calibration kit in all our measurement frequency range [100 MHz, 2 GHz].

### Estimation of the random error on the reflection coefficient via the SC

In total, our setup contains over 10 SMA-type connectors as well as cables of different lengths, ranging from 5 cm to 1 m. The impedance mismatch can lead to reflection coefficient differences of about -1dB and the cables act as $\lambda/2$ resonators. If the cable length coincides with resonances or anti-resonances ($l_{cable} = c/4f \simeq 50$ cm for a frequency $f$ = 1 GHz), a variation of -3 dB can be achieved with only three cables.

Moreover, the mechanical strength of the SMA connectors is not guaranteed during thermal cycling, leading to a non-reproducibility of the corresponding impedance mismatches between successive cool-downs.

### Data acquisition protocole

As explained in the main text, we measured the reflection coefficient while slowing ramping the temperature. However, the thermal ramp rates were slow enough (about 1 mK/min) so that no hysteresis were observed between warm-ups and cool-downs - meaning that the sample and the thermometer were well coupled thermally. The spectra acquisition time (in situ averaging of 10 spectra) was optimized for this thermal ramp rate and allowed to keep reasonable measurement duration (50 s for an averaged spectrum). The spectra shown were averaged from 10 raw spectra of closely spaced temperatures to reduce the random error on the reflection coefficient entering in the determination of the SBC calibration coefficients. Averaging was thus performed both during the measurement and offline.

### Weak localization corrections to the conductivity at $T_1$

The resistance versus temperature measurements show 2D weak localization features characterized by a relative increase of the resistance $\delta R/R \sim 0.1$. The theory of quantum correction to the electronic transport gives the relative increase of the impedance at low temperature in the low frequency limit:

$$\frac{\delta Z}{Z} = \frac{m}{\pi n_e h d}\frac{\ln(\tau_i/\tau_e)}{\tau_e}\left(1 + i\omega\frac{\tau_i}{\ln(\tau_i/\tau_e)}\right) \tag{1}$$

where $\tau_e$ and $\tau_i$ are the elastic and the inelastic lifetimes respectively [1]. The elastic lifetime is given by $\tau_e = l_e/v_F \simeq 8 \times 10^{-16}$ s. From the correction to the resistance and the normal resistance $R_n \simeq 25\,\Omega$, we extract $\tau_i \simeq 8 \times 10^{-11}$ s. We finally evaluate the imaginary part of the impedance at $T_1 \sim 400$ mK and $f = 2$ GHz, $\mathrm{Im}(Z(T_1)) \sim 9\,\mathrm{m}\Omega$ which is negligible compared to its real part $\mathrm{Re}(Z(T_1)) \sim 26\,\Omega$.

### Aslamazov-Larkin corrections to the conductivity at $T_1$ and $T_2$

For two-dimensional films as is the case here[2], the frequency dependence of the Aslamazov-Larkin correction to the conductivity is expressed as[3]: $\frac{\delta\sigma(T)}{\sigma_{DC}} = \left(\frac{2}{x}\tan^{-1}(x) - \frac{1}{x^2}\ln\left(1+x^2\right) - 1\right) + \mathrm{i}\left(\frac{2}{x}\left(\tan^{-1}(x) - x\right) - \frac{1}{x}\ln\left(1+x^2\right)\right)$ where $\sigma_{DC} = \frac{1}{16}\frac{e^2}{\hbar d}\frac{T_c}{T-T_c}$ is the DC Aslamazov-Larkin correction to the conductivity and $x = \frac{2\pi^2\hbar f}{16 k_B T_c}\frac{T_c}{T-T_c}$. In the considered frequency range [100 MHz, 2 GHz], we have $\frac{|\delta\sigma(T_1)|}{\sigma_{DC}} < 6 \times 10^{-3}$ and $\frac{|\delta\sigma(T_2)|}{\sigma_{DC}} < 5 \times 10^{-2}$.

### Value of the kinetic inductance at $T_3$

At low temperatures, it is reasonable that a-NbSi disordered thin films follow Mattis-Bardeen theory and that equation 4 of the manuscript is valid.

Indeed, penetration depth measurements have shown, in a similar system (a-$Mo_xGe_{1-x}$), that the BCS theory provided a good approximation for the measured kinetic inductance for $T < 0.9\ T_c$ [4].

Moreover, we have checked in a separate experiment involving resonators that a-NbSi films of similar compositions and thicknesses exhibited a kinetic inductance in line with the Mattis-Bardeen theory[5]


[1] G. Bergmann, Physical Review B **29**, 6114 (1984).

[2] F. Couëdo, O. Crauste, A.-A. Drillien, V. Humbert, L. Bergé, C. Marrache-Kikuchi, and L. Dumoulin, Scientific Reports **6** (2016).

[3] T. Ohashi, H. Kitano, A. Maeda, H. Akaike, and A. Fujimaki, Physical Review B **73**, 174522 (2006).

[4] S. J. Turneaure, T. R. Lemberger, and J. M. Graybeal, Physical Review Letters **84**, 987 (2000).

[5] G. Aiello, Private communication.
